# Supplementary material for: Question-Score Identity Detection (Q-SID): A Statistical Algorithm to Detect Collusion Groups with Error Quantification from Exam Question Scores
Source: arXiv:2407.07420 ancillary file (2024-07-12)
Supplement: Supplementary file 1 [file Q-SID Academic License.pdf]

# **Q-SID ACADEMIC LICENSE**

**July 2024**

## **1. DEFINITIONS**

### **1.1. “Contributor”**

means each individual or legal entity that creates, contributes to the creation of, or owns Covered Software.

### **1.2. “Contributor Version”**

means the combination of the Contributions of others (if any) used by a Contributor and that particular Contributor’s Contribution.

### **1.3. “Contribution”**

means Covered Software of a particular Contributor.

### **1.4. “Covered Software”**

means Source Code Form to which the initial Contributor has attached this License, the Executable Form of such Source Code Form, and Modifications of such Source Code Form, in each case including portions thereof.

### **1.5. “Executable Form”**

means any form of the work other than Source Code Form.

### **1.6. “Larger Work”**

means a work that combines Covered Software with other material, in a separate file or files, that is not Covered Software.

### **1.7. “License”**

means this document.

### **1.8. “Licensable”**

means having the right to grant, to the maximum extent possible, whether at the time of the initial grant or subsequently, any and all of the rights conveyed by this License.

### **1.9. “Modifications”**

means any of the following:

- a. any file in Source Code Form that results from an addition to, deletion from, or modification of the contents of Covered Software; or
- b. any new file in Source Code Form that contains any Covered Software.

#### **1.10. “Patent Claims” of a Contributor**

means any patent claim(s), including without limitation, method, process, and apparatus claims, in any patent Licensable by such Contributor that would be infringed, but for the grant of the License, by the making, using, selling, offering for sale, having made, import, or transfer of either its Contributions or its Contributor Version.

#### **1.11. “Other License”**

means any license other than this License. Other Licenses may be open or closed source.

#### **1.12. “Source Code Form”**

means the form of the work preferred for making modifications.

#### **1.13. “You” (or “Your”)**

means an individual or a legal entity exercising rights under this License. For legal entities, “You” includes any entity that controls, is controlled by, or is under common control with You. For purposes of this definition, “control” means (a) the power, direct or indirect, to cause the direction or management of such entity, whether by contract or otherwise, or (b) ownership of more than fifty percent (50%) of the outstanding shares or beneficial ownership of such entity.

#### **1.14 Non-Profit Educational Purposes**

means the use of the Covered Software for educational purposes at not for profit schools, colleges, universities or other teaching institutions, which use is not primarily intended for or directed towards commercial advantage or monetary compensation.

#### **1.15. Non-Commercial Research Purposes**

means the use of the Covered Software for academic research purposes or other not for profit or scholarly purposes, which use is not primarily intended for or directed towards commercial advantage or monetary compensation.

### **2. LICENSE GRANTS AND CONDITIONS**

#### **2.1. GRANTS**

Each Contributor hereby grants You a world-wide, royalty-free, non-exclusive license:

- a. under intellectual property rights (other than patent or trademark) Licensable by such Contributor to use, reproduce, make available, modify, display, perform, distribute, and otherwise exploit its Contributions, either on an unmodified basis, with Modifications, or as part of a Larger Work solely for Non-Profit Educational Purposes or Non-Commercial Research Purposes.
- b. under Patent Claims of such Contributor to make, practice and use its Contributions or its Contributor Version solely for Non-Profit Educational Purposes or Non-Commercial Research Purposes. This includes, but is not limited to, U.S. Patent No. 11,915,615 entitled “Systems and Methods for Detecting Collusion in Student Testing using Graded Scores or Answers for Individual Questions” granted to the initial Contributors.

## **2.2. EFFECTIVE DATE**

The licenses granted in Section 2.1 with respect to any Contribution become effective for each Contribution on the date the Contributor first distributes such Contribution.

## **2.3. LIMITATIONS ON GRANT SCOPE**

The licenses granted in this Section 2 are the only rights granted under this License. No additional rights or licenses will be implied from the distribution or licensing of Covered Software under this License. Notwithstanding Section 2.1(b) above, no patent license is granted by a Contributor:

- a. for any code that a Contributor has removed from Covered Software; or
- b. for infringements caused by: (i) Your and any other third party’s modifications of Covered Software, or (ii) the combination of its Contributions with other software (except as part of its Contributor Version); or
- c. under Patent Claims infringed by Covered Software in the absence of its Contributions.

This License does not grant any rights in the trademarks, service marks, or logos of any Contributor (except as may be necessary to comply with the notice requirements in Section 3.4).

## **2.4. FAIR USE**

This License is not intended to limit any rights You have under applicable copyright doctrines of fair use, fair dealing, or other equivalents.

## **2.5. CONDITIONS**

Sections 3.1, 3.2, 3.3, and 3.4 are conditions of the licenses granted in Section 2.1.

## **3. RESPONSIBILITIES**

### **3.1. DISTRIBUTION OF SOURCE FORM**

All distribution of Covered Software in Source Code Form, including any Modifications that You create or to which You contribute, must be under the terms of this License. You must inform recipients that the Source Code Form of the Covered Software is governed by the terms of this License, and provide them with a copy of this License. You may not attempt to alter or restrict the recipients' rights in the Source Code Form.

### **3.2. DISTRIBUTION OF EXECUTABLE FORM**

If You distribute Covered Software in Executable Form then:

- a. such Covered Software must also be made available in Source Code Form, as described in Section 3.1, and You must inform recipients of the Executable Form how they can obtain a copy of such Source Code Form by reasonable means in a timely manner at no cost to the recipient; and
- b. You must distribute such Executable Form under the terms of this License and provide recipients with a copy of this License.

### **3.3. DISTRIBUTION OF A LARGER WORK**

You may create and distribute a Larger Work under terms of Your choice, provided that You also comply with the requirements of this License for the Covered Software, including the terms in 2.1.a and 2.1.b governing permissible purposes. If the Larger Work is a combination of Covered Software with a work governed by one or more Other Licenses, the Covered Software must be distributed in a separate file under the terms of this License, not the terms of the Other Licenses.

### **3.4. NOTICES**

You may not remove or alter the substance of any license notices (including copyright notices, patent notices, disclaimers of warranty, or limitations of liability) contained within the Source Code Form of the Covered Software, except that You may alter any license notices to the extent required to remedy known factual inaccuracies.

## **4. INABILITY TO COMPLY DUE TO STATUTE OR REGULATION**

If it is impossible for You to comply with any of the terms of this License with respect to some or all of the Covered Software due to statute, judicial order, or regulation then You must: (a) comply with the terms of this License to the maximum extent possible; and (b) describe the limitations and the code they affect. Such description must be placed in a text file included with all distributions of the Covered Software under this License. Except to the extent prohibited by statute or regulation, such description must be sufficiently detailed for a recipient of ordinary skill to be able to understand it.

## **5. TERMINATION**

5.1. The rights granted under this License will terminate automatically if You fail to comply with any of its terms. However, if You become compliant, then the rights granted under this License from a particular Contributor are reinstated (a) provisionally, unless and until such Contributor explicitly and finally terminates Your grants, and (b) on an ongoing basis, if such Contributor fails to notify You of the noncompliance by some reasonable means prior to 60 days after You have come back into compliance. Moreover, Your grants from a particular Contributor are reinstated on an ongoing basis if such Contributor notifies You of the non-compliance by some reasonable means, this is the first time You have received notice of non-compliance with this License from such Contributor, and You become compliant prior to 30 days after Your receipt of the notice.

5.2. If You initiate litigation against any entity by asserting a patent infringement claim (excluding declaratory judgment actions, counterclaims, and cross-claims) alleging that a Contributor Version directly or indirectly infringes any patent, then the rights granted to You by any and all Contributors for the Covered Software under Section 2.1 of this License shall terminate.

5.3. In the event of termination under Sections 5.1 or 5.2 above, all end user license agreements (excluding distributors and resellers) which have been validly granted by You or Your distributors under this License prior to termination shall survive termination.

## **6. DISCLAIMER OF WARRANTY**

Covered Software is provided under this License on an “as is” basis, without warranty of any kind, either expressed, implied, or statutory, including, without limitation, warranties that the Covered Software is free of defects, merchantable, fit for a particular purpose or non-infringing. The entire risk as to the quality and performance of the Covered Software is with You. Should any Covered Software prove defective in any respect, You (not any Contributor) assume the cost of any necessary servicing, repair, or correction. This disclaimer of warranty constitutes an essential part of this License. No use of any Covered Software is authorized under this License except under this disclaimer.

## **7. LIMITATION OF LIABILITY**

Under no circumstances and under no legal theory, whether tort (including negligence), contract, or otherwise, shall any Contributor, or anyone who distributes Covered Software as permitted above, be liable to You for any direct, indirect, special, incidental, or consequential damages of any character including, without limitation, damages for lost profits, loss of goodwill, work stoppage, computer failure or malfunction, or any and all other commercial damages or losses, even if such party shall have been informed of the possibility of such damages. This limitation of liability shall not apply to liability for death or personal injury resulting from such party’s negligence to the extent applicable law prohibits such limitation.

Some jurisdictions do not allow the exclusion or limitation of incidental or consequential damages, so this exclusion and limitation may not apply to You.

## **8. LITIGATION**

Any litigation relating to this License may be brought only in the courts of a jurisdiction where the defendant maintains its principal place of business and such litigation shall be governed by laws of that jurisdiction, without reference to its conflict-of-law provisions. Nothing in this Section shall prevent a party's ability to bring cross-claims or counter-claims.

## **9. MISCELLANEOUS**

This License represents the complete agreement concerning the subject matter hereof. If any provision of this License is held to be unenforceable, such provision shall be reformed only to the extent necessary to make it enforceable. Any law or regulation which provides that the language of a contract shall be construed against the drafter shall not be used to construe this License against a Contributor.
