# Supplementary material for: Question-Score Identity Detection (Q-SID): A Statistical Algorithm to Detect Collusion Groups with Error Quantification from Exam Question Scores
Source: arXiv:2407.07420 ancillary file (2024-07-12)

# Question-Score Identity Detection (Q-SID) Version 2.2, November 2022

## What Q-SID does

Q-SID identifies groups of students whose question scores on an exam are more similar to each other than is usual. Using this information, the course instructor can then compare the written answers of students within each identified group to determine if this similarity is due to collusion.

Q-SID was developed in response to the increase in cheating when the COVID-19 pandemic prevented strict, in-person proctoring of exams. In several STEM classes at UC Berkeley, for example, 1% - 19% of students were found to have colluded in open book exams taken by students in their homes without proctoring. Students typically colluded in groups of two to five. Forensic examination of written answers showed that within each group information had been exchange for many but not all questions. Most of these students confessed to cheating when challenged. Such validated exam data has been used to develop Q-SID along with feedback from course instructors.

Q-SID requires only scores from each question and each student's total score on the exam. It is thus applicable to many exam formats. The question scores may be either numeric values—representing the graded number of points that the student obtained—or for multiple choice questions any one letter/word of text representing students' answers: for example a, b, c, d, or e; or true or false. Q-SID does not compare longer text or other details of an exam. Instead, each student is given a Collusion Score (CS) that defines the similarity of their exam to that of the partner in the class that shares the highest number of identical question scores. The student/partner pair with the largest CS is the pair most likely to have colluded.

## Collusion Groups

Because students often collude in groups larger than two, Q-SID clusters student/partner pairs who share members into Collusion Groups. Collusion Group membership is limited to pairs with high CSs, and the groups are ranked by CS.

The figure right shows the Collusion Groups identified in two unproctored exams from a class of 263 students. Most students who colluded did so on both exams. All but two of the forty six students placed by Q-SID into Collusion Groups are known to have colluded based on their written answers and/or confessions. Six other students who colluded in this class had CSs below the thresholds used to form Collusion Groups. For this class, Q-SID therefore identified 88% of the students who colluded while finding two false positives.

| EXAM 1 |        |        |     |      | EXAM 2 |        |        |     |      |
|--------|--------|--------|-----|------|--------|--------|--------|-----|------|
| Group  | empFPR | synFPR | ID  | CS   | Group  | empFPR | synFPR | ID  | CS   |
| 1      | 0.04%  | 0.09%  | 133 | 2.42 | 2      | 0.04%  | 0.13%  | 183 | 2.61 |
| 1      | 0.04%  | 0.09%  | 166 | 2.33 | 2      | 0.04%  | 0.13%  | 170 | 2.33 |
| 1      | 0.04%  | 0.09%  | 137 | 2.31 | 7      | 0.04%  | 0.13%  | 234 | 2.44 |
| 2      | 0.04%  | 0.09%  | 170 | 2.42 | 7      | 0.04%  | 0.13%  | 226 | 2.33 |
| 2      | 0.04%  | 0.09%  | 183 | 2.33 | 6      | 0.04%  | 0.13%  | 228 | 2.40 |
| 2      | 0.04%  | 0.09%  | 193 | 1.93 | 6      | 0.04%  | 0.13%  | 218 | 2.11 |
| 3      | 0.04%  | 0.09%  | 221 | 2.11 | 12     | 0.04%  | 0.13%  | 237 | 2.33 |
| 3      | 0.04%  | 0.09%  | 227 | 1.93 | 12     | 0.04%  | 0.13%  | 222 | 2.20 |
| 4      | 0.04%  | 0.09%  | 124 | 2.00 | 11     | 0.04%  | 0.13%  | 224 | 2.33 |
| 4      | 0.04%  | 0.09%  | 142 | 1.92 | 11     | 0.04%  | 0.13%  | 192 | 1.89 |
| 4      | 0.04%  | 0.09%  | 122 | 1.67 | 1      | 0.04%  | 0.13%  | 133 | 2.09 |
| 4      | 0.04%  | 0.09%  | 98  | 1.62 | 1      | 0.04%  | 0.13%  | 166 | 2.00 |
| 5      | 0.04%  | 0.09%  | 187 | 2.00 | 1      | 0.04%  | 0.13%  | 137 | 1.82 |
| 5      | 0.04%  | 0.09%  | 150 | 1.67 | 9      | 0.04%  | 0.13%  | 185 | 1.89 |
| 6      | 0.04%  | 0.09%  | 218 | 1.86 | 9      | 0.04%  | 0.13%  | 151 | 1.32 |
| 6      | 0.04%  | 0.09%  | 228 | 1.69 | 3      | 0.04%  | 0.13%  | 221 | 1.71 |
| 7      | 0.04%  | 0.09%  | 226 | 1.80 | 3      | 0.04%  | 0.13%  | 172 | 1.70 |
| 7      | 0.04%  | 0.09%  | 234 | 1.69 | 16     | 0.20%  | 0.31%  | 208 | 1.67 |
| 8      | 0.04%  | 0.09%  | 89  | 1.79 | 16     | 0.20%  | 0.31%  | 209 | 1.60 |
| 8      | 0.04%  | 0.09%  | 88  | 1.71 | 17     | 0.20%  | 0.31%  | 149 | 1.64 |
| 8      | 0.04%  | 0.09%  | 84  | 1.71 | 17     | 0.20%  | 0.31%  | 150 | 1.64 |
| 8      | 0.04%  | 0.09%  | 91  | 1.38 | 15     | 0.56%  | 0.65%  | 180 | 1.55 |
| 8      | 0.04%  | 0.09%  | 65  | 1.36 | 15     | 0.56%  | 0.65%  | 177 | 1.33 |
| 9      | 0.04%  | 0.09%  | 185 | 1.75 | 14     | 0.56%  | 0.65%  | 25  | 1.54 |
| 9      | 0.04%  | 0.09%  | 151 | 1.67 | 14     | 0.56%  | 0.65%  | 55  | 1.52 |
| 9      | 0.04%  | 0.09%  | 182 | 1.33 | 14     | 0.56%  | 0.65%  | 168 | 1.33 |
| 10     | 0.20%  | 0.23%  | 163 | 1.62 | 18     | 0.56%  | 0.65%  | 99  | 1.50 |
| 10     | 0.20%  | 0.23%  | 108 | 1.42 | 18     | 0.56%  | 0.65%  | 202 | 1.33 |
| 11     | 0.56%  | 0.62%  | 192 | 1.57 |        |        |        |     |      |
| 11     | 0.56%  | 0.62%  | 224 | 1.50 |        |        |        |     |      |
| 12     | 0.56%  | 0.62%  | 222 | 1.57 |        |        |        |     |      |
| 12     | 0.56%  | 0.62%  | 237 | 1.47 |        |        |        |     |      |
| 13     | 0.56%  | 0.62%  | 160 | 1.55 |        |        |        |     |      |
| 13     | 0.56%  | 0.62%  | 154 | 1.50 |        |        |        |     |      |
| 14     | 0.56%  | 0.62%  | 55  | 1.53 |        |        |        |     |      |
| 14     | 0.56%  | 0.62%  | 25  | 1.31 |        |        |        |     |      |
| 15     | 0.56%  | 0.62%  | 180 | 1.50 |        |        |        |     |      |
| 15     | 0.56%  | 0.62%  | 105 | 1.42 |        |        |        |     |      |

## False Positive Rates

To estimate the fraction of students placed into Collusion Groups who did NOT collude, each group is assigned an Empirical False Positive Rate (FPR) and in many cases also a Synthetic FPR.

Empirical FPRs are the percent of students from 36 proctored exams who have CSs above or between one of three CS thresholds that divide Collusion Groups into three so called FPR bins. The 10,816 students who took the 36 in-person proctored exams are assumed not to have colluded. Thus the frequencies of students in an instructor's exam whose CSs fall within the three FPR bins estimate the percent of students in that exam who have NOT colluded but who will nonetheless be placed into one of more of the FPR bins. The three standard CS thresholds have been chosen to correspond to cumulative Empirical FPRs of 0.04%, 0.20% and 0.56%. Thus—as examples—in an exam taken by 357 students one would expect on average one pair of students who did NOT collude to be placed into a Collusion Group, most likely in the 0.56% FPR bin. In exams taken by 500 students each, one would expect a pair of false positives in the 0.04% FPR bin only in one out of every ten exams.

Synthetic FPRs are calculated from *in silico* generated exam results tailored for the Instructor's exam. The *in silico* data are produced to have an identical number of students and questions as the instructor's query exam as well as similar distributions of numeric scores for each question and total scores on the exam. Importantly, the *in silico* results are generated such that the question scores for each individual student are independent of those of the other students in the class. The *in silico* data, thus, mimic the case where there is no collusion. Multiple synthetic exams are produced to give data for just over 100,000 students. The *in silico* data are then analyzed by Q-SID, which assigns students to three FPR bins using the same three CS thresholds used to define the Empirical FPR bins. The Synthetic FPRs are simply the percent of students from the total set of synthetic exams who are assigned to each of the three FPR bins.

For each of the three Empirical FPRs there is thus a corresponding Synthetic FPR. The former are constant for all exams, whereas the latter vary between exams. Though the two FPRs are calculated using entirely different data and assumptions, they broadly agree. In rare the instances when a Synthetic FPR exceeds 0.8%, such Collusion Groups are not reported. In the current implementation of Q-SID, though, Synthetic FPRs are not calculated when non-numeric question score data is present, such as true or false or a, b, c, d, or e.

The histograms to the right compare the distribution of CSs for one of the unproctored exams from page 1 (query exam, green) to that of the corresponding CS data used to determine the Empirical FPR (top, red) and the Synthetic FPR (bottom, yellow). Fewer students have high CSs in the Empirical and Synthetic control exams than in the unproctored query exam, consistent with the independent evidence than tens of students colluded in this exam. No specific CS, however, cleanly separates all students who collude from those that do not. For example

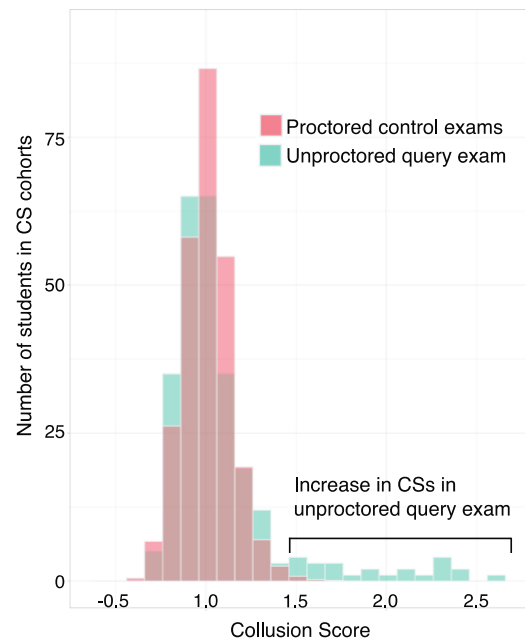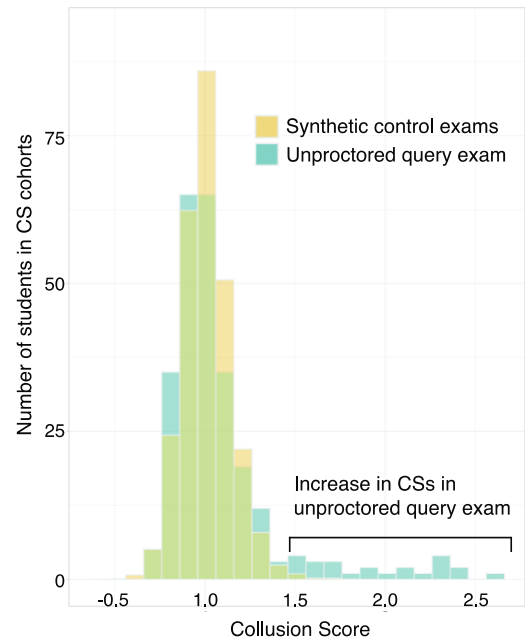

in the plots, some students with CSs of 1.5 will likely have colluded, but others may not have and for this reason CS alone cannot be used to determine if students have colluded.

The bar and whisker plots, right, illustrate that FPRs are much lower than the percent of students who colluded in unproctored exams at UC Berkeley and UCLA. The percent of students placed into each of the three FPR bins in 34 unproctored exams (green, 10,526 individual tests) is compared to the percentages found in the Synthetic controls for these exams (yellow > 3,400,000 individual tests) and the 36 proctored control exams used to determine the Empirical FPR (red, 10,816 individual tests). The bins are named by their cumulative Empirical FPRs: i.e. 0.04%, 0.20% and 0.56%. Approximately half of all students placed into Collusion Groups in unproctored exams are found in the 0.05% FPR bin (2.4% of students who took the exams), whereas very few students in the proctored, Empirical control exams or in the Synthetic control exams are placed in this FPR bin. For the 0.20% and 0.56% FPR bins, more students are identified in unproctored exams than in the Empirical and Synthetic controls, but the discrimination is not as clear cut as for 0.04% FPR bin.

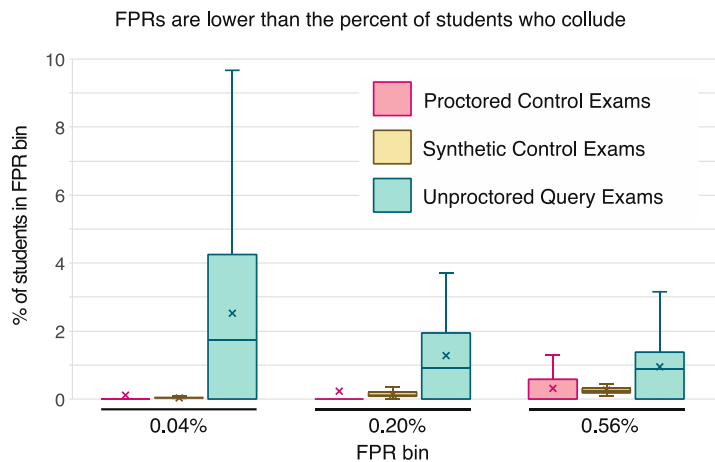

### Deterring Collusion

Q-SID can deter Collusion. The bar and whisker plots below show the percent of students assigned to Collusion Groups (y-axis) in exams from classes of the same UC Berkeley course. Twenty two exams were given as traditional, in-person proctored exams in the three years prior to the pandemic (red). After the onset of the pandemic all exams were given online without proctoring. For five of these unproctored exams, students were not aware that Q-SID would be used to detect collusion (light green). For another nine unproctored exams, students were either shown the Q-SID website or were informed that others in their class had been caught cheating using Q-SID (dark green).

Prior to each unproctored exam, Students were reminded of the honor code and signed a statement attesting that they would not collude. Despite this, in those exams shortly after the onset of the pandemic 7% – 14% of students colluded. To more effectively dissuade students from cheating, in subsequent unproctored exams students were clearly informed about Q-SID prior to taking their exams. The percentages of students who colluded in these cases were 2% - 7%. Informing students about Q-SID reduced collusion by several fold on average. To assist in persuading students, the Q-SID website includes a special page addressed to students explaining that Q-SID's purpose is to protect the grades of the large majority of students who do not cheat and to help those considering colluding not to do so. Most of the students who ignored this advice and colluded despite being informed about Q-SID confessed to cheating when challenged and indicated that in future they would not cheat. While these latter cases are not ideal, deterrence by being sanctioned is an additional mechanism by which Q-SID dissuades students from colluding in subsequent classes.

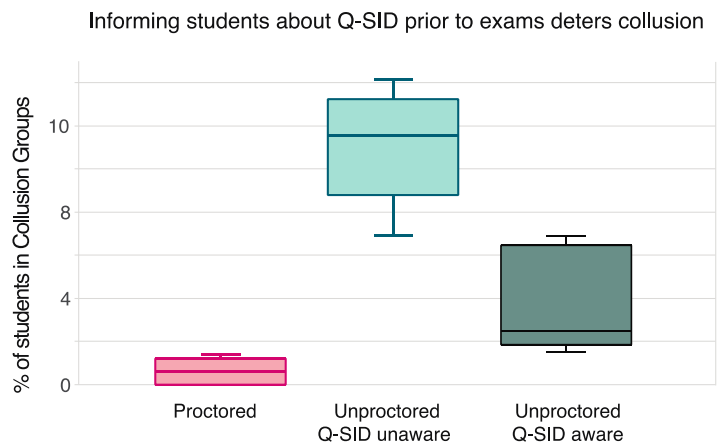

## Manual comparison of written answers

Q-SID's FPRs are only a guide to the likelihood that students in a given Collusion Group have colluded. To determine which specific students in fact have colluded, the written answers of Collusion Groups members must be manually compared. Collusion can be quickly ruled out for students who have not cheated by comparing their written answers. In our experience, a lack of similarity in detail is readily apparent. For Collusion Groups where answer text appears similar on a first pass through the exam, a more time consuming process is then required. This involves first finding unlikely or unusual aspects of the suspects answers to specific questions, then looking at all other students' answers. Where students have colluded, at least several examples can be found for which the only students giving a particular answer are the members of that group.

For multiple choice only exams, which lack detailed written answers, Q-SID should only be used to gauge if collusion has occurred, not to identify and challenge specific students suspected of cheating. When collusion is found in such exams, instructors should consider alternate exam formats or improved proctoring in future.

## Exam design and Q-SID performance

### Number of question scores

Q-SID performance is strongly influenced by the number of question scores. True positives are defined as students shown to have colluded based on detailed examination of written exam answers. Randomly sampled subsets of question scores were drawn from one of the unproctored example exams from page 1. The figure right shows that only 10% of true positives are identified using 20 question scores, but 50% of true positives are captured with 60 question scores and 80% with 83 scores. In addition, we have found that the distribution of CSs can be unreliable with <20 question scores. Therefore, Q-SID will not process exam data with fewer than 20 question scores.

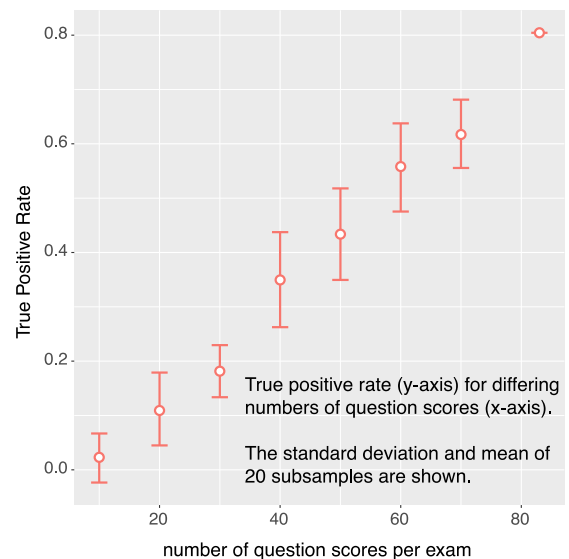

### Number of exams

Increasing the number of exams analyzed can improve Q-SID performance in two ways.

First, analyzing each exam from the same class separately increases the percent of students detected. In the example exams shown on page 1, while most groups who colluded in Exam 1 also colluded within the same group in Exam 2, several of the true positives not identified in the Collusion Groups for Exam 1 were in the Collusion Groups reported for Exam 2 and *vice versa*.

Second, the figure right shows that Q-SID can combine data from two or more exams in a single analysis to obtain a higher true positive rate. For example, Q-SID performance is lowest using either 30 questions subsampled from Exam 1 or 30 questions subsampled from Exam 2. Performance is improved by analyzing scores from 60 questions, 30 from each of the two subsamples (Exam1&2 30+30).

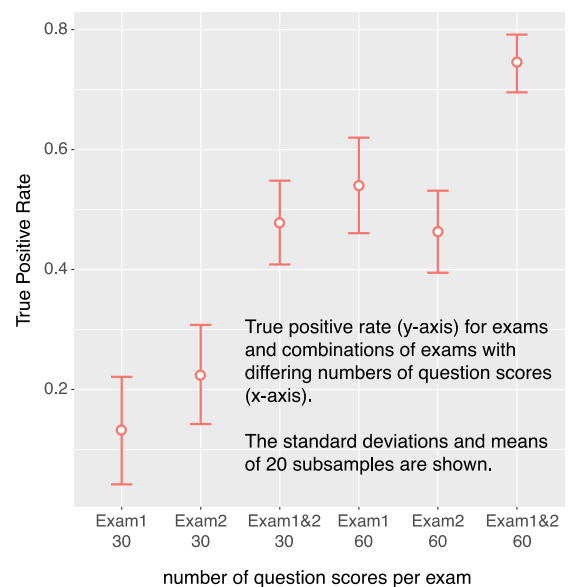

### Question score Complexity

In addition to being affected by the number of question scores, Q-SID performance is influenced by the frequency at which the class obtain similar or different scores on each question. Instructors differ in the style of exams that they set. At one extreme a confirmatory exam may be set in which most questions are answered correctly by almost all members of the class. As a result most students will have similar scores for each question. Alternatively, in a more rigorous test students may obtain a wide spread of scores for each question. Questions that give the greatest discrimination between students are more powerful for detecting collusion. For example, analysis of the 50 questions with the smallest variation in scores among students from a particular class identified only 7% of true positives. By contrast, analysis of the 50 questions with the largest variation in scores from this class identified 56% of true positives.

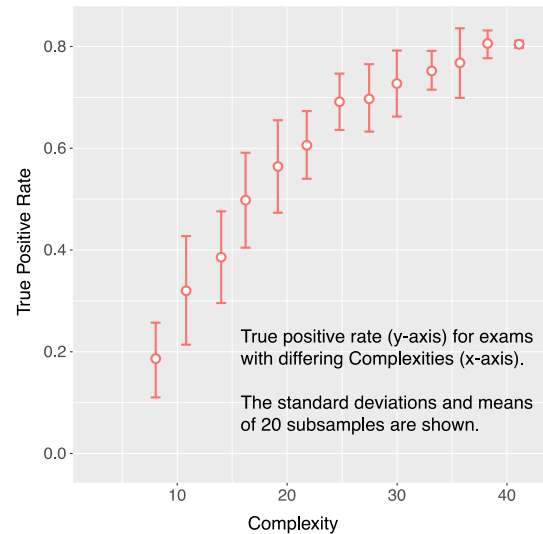

To account for both the number of questions and the discriminatory power of each question, Q-SID calculates a Complexity value for each exam. The figure top right shows the percent of true positives identified for sets of questions with an array of Complexities. This plot can be used as a guide to the likely performance of Q-SID for classes of 100 or more students.

For technical reasons, Q-SID is not effective for exams with Complexities <8 and will not calculate CSs for exams below this threshold. We recommend that exams have a Complexity of  $\geq 15$ . For exams whose Complexity is less than this ideal, we recommended that two or more exams from the same class exams be combined. The Complexity of combined exams can be simply calculated by summing of the Complexities of the individual exams. To further maximize exam Complexity, when some questions carry many points, instructors should breakdown and recoded separately the scores for parts of the question to generate more independent scores. If a subset of questions on the test are multiple choice, record the students choice of answer as a Question Score. Knowing which wrong answer students give increases Complexity and thus provides additional statistical power in detecting collusion.

To predict the likely Complexity of a new exam prior to it being given, instructors can use Q-SID to analyze prior exams for their class which have a similar number and style of question. As a guide, the mean Complexity per question we have observed in exams is 0.33 with a minimum of 0.16 and a maximum of 0.65. Achieving a Complexity of 15 will usually require at least 40 question scores.

### Number of students

Q-SID is effective for classes of 25 or more students. Randomly selected subsamples of between 25 to 250 students were used to model different size classes. The figure right shows that there is little variation in the percent of true positives identified for classes of 100 or more students. For classes progressively smaller than 100, the true positive rate reduces, but remains useful. The lower limit for the number of exam participants that Q-SID will accept is 25.

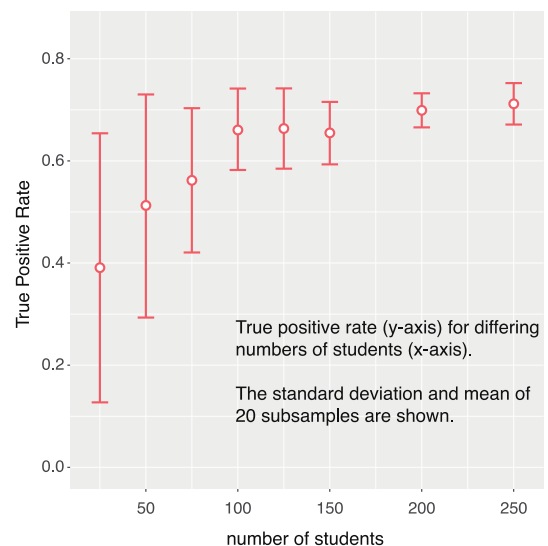



## Input and output files

### *Input file*

On the Q-SID web site's Analyze Data page, the user enters the course name, the exam(s) name, and the number of exams. These entries will be used by Q-SID to label the output report files.

The user is then asked to upload an excel file in either .xls, .xlsx or .csv formats. When uploading a single exam for analysis, the data should be placed on Sheet 1. When uploading multiple exams for the same class for a combined analysis, each exam should be placed on a separate sheet in the file, starting with Sheet 1 and with subsequent exams placed on consecutive sheets. Q-SID expects the number of exams specified by the user to correspond to the number of sheets with data. When more than one exam is included, Q-SID combines and uses data only for those students whose IDs are present in all exams.

On each sheet, the top row should describe the information in each column for all rows below it. The user chooses which titles to use for these column headers, but the titles must correspond to the information specified below.

The columns in the second and successive rows must contain in order left to right: the student's ID, which can be any text; the student's total score on the exam, which must be a number; and multiple columns, each of which give the score for one question. The question score may be either a numeric value—representing the graded number of points that the student obtained—or for multiple choice questions any one letter/word of text representing the student's choice of answer, for example a, b, c, d or e; or true or false. Each row must contain information for one student. Data from any rows that share the same Student ID as well as data in any row lacking an ID will be not be used by Q-SID. Q-SID will list the IDs of any data it ignores.

The columns and rows must be in the order specified. Ensure that no additional information is present in the file below the rows containing student data. A template excel file can be downloaded from the Q-SID website as an example.

### *Output files*

Q-SID delivers two files.

**1. An output excel file**, the second and successive rows of which each list the information for one student/partner pair. Columns list a variety of information including if the student belongs to a Collusion Group; the group's Empirical and Synthetic FPRs; the IDs of the student and their partner; the pair's CS and CS rank; the student's test score and test score rank; as well as further information on the partner. Where more than one exam is provided, the students' test scores are the sum of their test scores entered for each exam. In addition, a second partner is defined who has the second highest number of identical question scores with the student. Information on this second partner is also provided as it is used by the clustering method to sort students into Collusion Groups. A list of the order of columns is given in the Appendix. The rows are ranked by CS and Collusion Group.

**2. A report pdf file** that displays on successive pages.

- Histograms of the CSs of the query exam compared to histograms of CSs for the Empirical and Synthetic controls.
- A list of the Collusion Groups, their Empirical and Synthetic FPRs with 95% confidence limits, the IDs of their members and their CSs.
- A bar graph of the CSs, ordered by the students' test score rank.
- For every Collusion Group, a histogram of the number of question scores identical between a designated member of the group and each other student in the class. The group member with the highest CS is designated.

An example report pdf file is provided in the Appendix

## **APPENDIX**

1. List of columns in Q-SID output excel file.
2. List of possible advice messages provided on page 2 of the Q-SID Report pdf.
3. Example Q-SID Report pdf.

## 1. Order of columns in Q-SID output excel file

|                                                   |
|---------------------------------------------------|
| Collusion Group                                   |
| Empirical FPR                                     |
| Synthetic FPR                                     |
| Student ID                                        |
| Test Score (TS) <sup>1</sup>                      |
| TS Rank                                           |
| Collusion Score (CS)                              |
| CS Rank                                           |
| 1st Partner ID <sup>2</sup>                       |
| Identity Score (IS) with 1st Partner <sup>3</sup> |
| 1st Partner CS                                    |
| 2nd Partner ID <sup>4</sup>                       |
| IS with 2nd Partner                               |
| 2nd Partner CS                                    |

<sup>1</sup> Test Score is the total score a student obtained on the exam

<sup>2</sup> The 1st partner is the student in the class with whom a student shares the highest IS.

<sup>3</sup> Identity Score is the number of questions for which a pair of students obtain the identical score

<sup>4</sup> The 2nd partner is the student in the class with whom a student shares the next to highest IS.



## 2. Advice messages provided in the Q-SID report

Page 1 or 2 of the Q-SID report may include one or more of the following advice messages when the input data file is suboptimal.

### On page 1: CSs are not calculated

For an exam or combination of exams with Complexity < 8 or # question scores < 20, CSs are not calculated, Collusion Groups are not listed and the output excel file is withheld. The following advice message is given:

The query exam(s) have too few question scores and/or too low a Complexity to reliably determine collusion. Q-SID requires a minimum of 20 question scores and a Complexity of at least 8. Please see the Q-SID guide for suggestions on increasing the number of question scores and exam Complexity, including combining multiple exams from the same class. Ideally, an exam or combination of exams should have at least 50 question scores and a Complexity of 15 or more.

For an exam defined by the user as only containing numeric question scores and for which non-numeric characters or no data are found for some question scores, CSs are not calculated, Collusion Groups are not listed and the output excel file is withheld. The following advice message is given:

One or more non-numeric characters or blank entries are present for some questions. If the input file contains multiple choice answers, please resubmit the file by answering no to the question "Only numeric question scores?" on the Analyze Data page. If the input file is intended to contain only contain numeric question scores, please correct the non-numeric entries. The following questions contained non-numeric characters.

## "column header here"

## "column header here"

For an exam or combination of exams with mean Complexity / question >1, CSs are not calculated, Collusion Groups are not listed and the output excel file is withheld. The following advice message is given:

The query exam(s)' Complexity per question is too high to reliably determine collusion. The number of possible question scores per question is much higher than is typical for exams. Please check the input data file as this could reflect an error in the file.

### On page 2: CSs are calculated

For an exam with either replicated student IDs or rows lacking a student ID, data for all such rows is ignored in calculating CSs. The Collusion Groups and other standard Q-SID outputs are provided for the remaining student's data, together with the following advice message:

Two or more rows in the input data have identical student IDs, or one or more rows have no ID. All such data were removed prior to analysis. Please correct the input data and reanalyze to ensure a complete result. The data removed had the following IDs

## [1] "ID or blank here"

## [2] "ID or blank here"

For an exam or combination of exams with  $8 \leq \text{Complexity} < 15$ , Collusion Groups and other standard Q-SID outputs are provided together with the following advice message:

Your query exam(s)' Complexity is lower than ideal to maximally detect Collusion. Ideally the Complexity of exams should be at least 15. Please see the Q-SID guide for suggestions on increasing the number of question scores and exam Complexity, including combining multiple exams from the same class.

In rare cases the Synthetic FPR for one or more of the FPR bins will exceed 0.8%. In these cases, Collusion Groups for these FPR bins will not be listed, but FPR bins with lower Synthetic FPRs will still be reported with the following advice message:

One or more of the FPR bins had a Synthetic FPR > 0.8%. Collusion Groups for these FPR bins have been omitted.

For exam data that includes multiple choice answers for one of more questions, Q-SID does not calculate a Synthetic FPR. The following advice message is displayed.

No Synthetic FPR is provided as Q-SID currently does not calculate these FPRs in cases where multiple choice answers are included in the input data.

# Q-SID REPORT

**Course:** Benchmark

**Numeric questions scores only?** Yes

**Query Exam:** Exam1

**# Students:** 269

**# Exams:** 1

**# Questions:** 83

**Complexity:** 25.2

## 1. The distribution of Collusion Scores (CSs) in the query exam(s) compared to those for two independent negative controls: an Empirical Control and a Synthetic Control

Each student is assigned a CS based on the maximum number of identical question scores that they share with another student in the class. Query Exams that have suffered significant collusion have more students with high CS values compared to both negative controls.

A. left, the Empirical Control is the distribution of CSs from multiple strictly proctored real exams in which students are presumed not to have colluded. For query exams with <250 students, the real exam data is down sampled to approximate the number of students in the query exam.

B. right, the Synthetic Control is the distribution of CSs from many in silico exams that combined represent over 100,000 students. Each in silico exam replicates the number of students and questions for the query exam and closely approximates the distributions of question and test scores. The in silico question scores of each student are generated such that they are independent of those of other individual students.

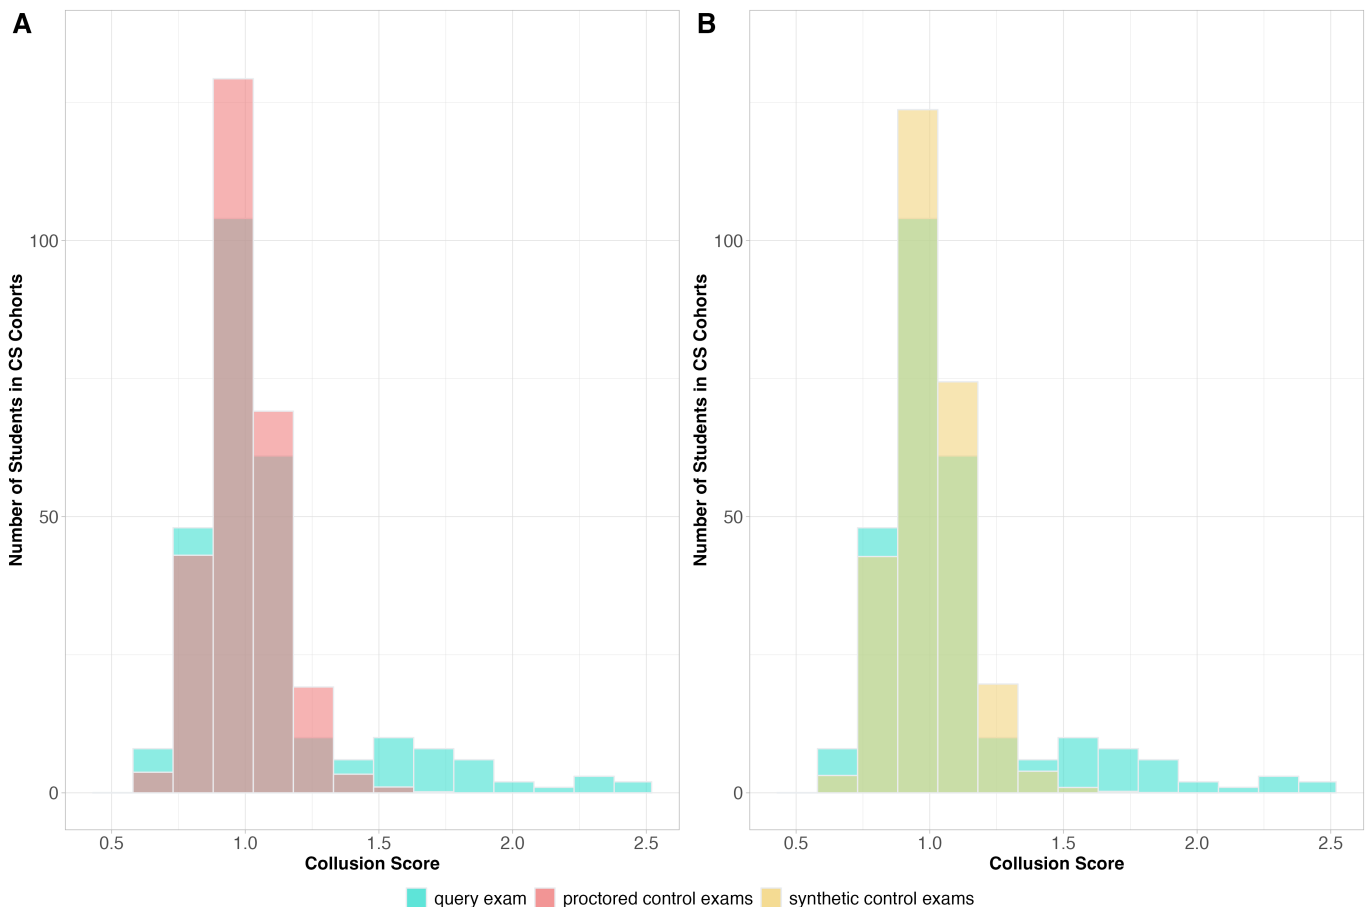

## 2. Table for Collusion Groups

Students are arranged into groups based on higher than usual identity in question scores on their exams. The resulting Collusion Groups are ranked by the CS of the group member with the largest CS. Each Collusion Group is assigned two independently derived false positive rates (FPRs) based on the percentage of students that are found with similarly high CSs in the Empirical Control or in the Synthetic Control.

Collusion Group membership is not direct evidence of collusion. The written exam answers of group members must be examined in detail to determine if collusion has occurred, see the Q-SID guide for further explanation.

| Group | empFPR | synFPR | ID  | CS   |
|-------|--------|--------|-----|------|
| 1     | 0.04%  | 0.09%  | 133 | 2.42 |
| 1     | 0.04%  | 0.09%  | 166 | 2.33 |
| 1     | 0.04%  | 0.09%  | 137 | 2.31 |
| 2     | 0.04%  | 0.09%  | 170 | 2.42 |
| 2     | 0.04%  | 0.09%  | 183 | 2.33 |
| 2     | 0.04%  | 0.09%  | 193 | 1.93 |
| 3     | 0.04%  | 0.09%  | 221 | 2.11 |
| 3     | 0.04%  | 0.09%  | 227 | 1.93 |
| 4     | 0.04%  | 0.09%  | 124 | 2.00 |
| 4     | 0.04%  | 0.09%  | 142 | 1.92 |
| 4     | 0.04%  | 0.09%  | 122 | 1.67 |
| 4     | 0.04%  | 0.09%  | 98  | 1.62 |
| 5     | 0.04%  | 0.09%  | 187 | 2.00 |
| 5     | 0.04%  | 0.09%  | 150 | 1.67 |
| 6     | 0.04%  | 0.09%  | 218 | 1.86 |
| 6     | 0.04%  | 0.09%  | 228 | 1.69 |
| 7     | 0.04%  | 0.09%  | 226 | 1.80 |
| 7     | 0.04%  | 0.09%  | 234 | 1.69 |
| 8     | 0.04%  | 0.09%  | 89  | 1.79 |
| 8     | 0.04%  | 0.09%  | 88  | 1.71 |
| 8     | 0.04%  | 0.09%  | 84  | 1.71 |
| 8     | 0.04%  | 0.09%  | 91  | 1.38 |
| 8     | 0.04%  | 0.09%  | 65  | 1.36 |
| 9     | 0.04%  | 0.09%  | 185 | 1.75 |
| 9     | 0.04%  | 0.09%  | 151 | 1.67 |
| 9     | 0.04%  | 0.09%  | 182 | 1.33 |
| 10    | 0.20%  | 0.23%  | 163 | 1.62 |
| 10    | 0.20%  | 0.23%  | 108 | 1.42 |
| 11    | 0.56%  | 0.62%  | 192 | 1.57 |
| 11    | 0.56%  | 0.62%  | 224 | 1.50 |
| 12    | 0.56%  | 0.62%  | 222 | 1.57 |
| 12    | 0.56%  | 0.62%  | 237 | 1.47 |
| 13    | 0.56%  | 0.62%  | 160 | 1.55 |
| 13    | 0.56%  | 0.62%  | 154 | 1.50 |
| 14    | 0.56%  | 0.62%  | 55  | 1.53 |

|    |       |       |     |      |
|----|-------|-------|-----|------|
| 14 | 0.56% | 0.62% | 25  | 1.31 |
| 15 | 0.56% | 0.62% | 180 | 1.50 |
| 15 | 0.56% | 0.62% | 105 | 1.42 |

The 95% confidence limits for the FPRs are as follows.

| FPR Bin | Empirical FPR       | Synthetic FPR       |
|---------|---------------------|---------------------|
| 0.04%   | 0.037% (+/- 0.036%) | 0.086% (+/- 0.018%) |
| 0.20%   | 0.203% (+/- 0.085%) | 0.228% (+/- 0.030%) |
| 0.56%   | 0.555% (+/- 0.140%) | 0.621% (+/- 0.049%) |

3. Bar Graph of CSs Ranked by Student Test Score

Students are arranged by test score, with the highest scoring student to the left, rank = 1. The height of the bars show the CS for each student.

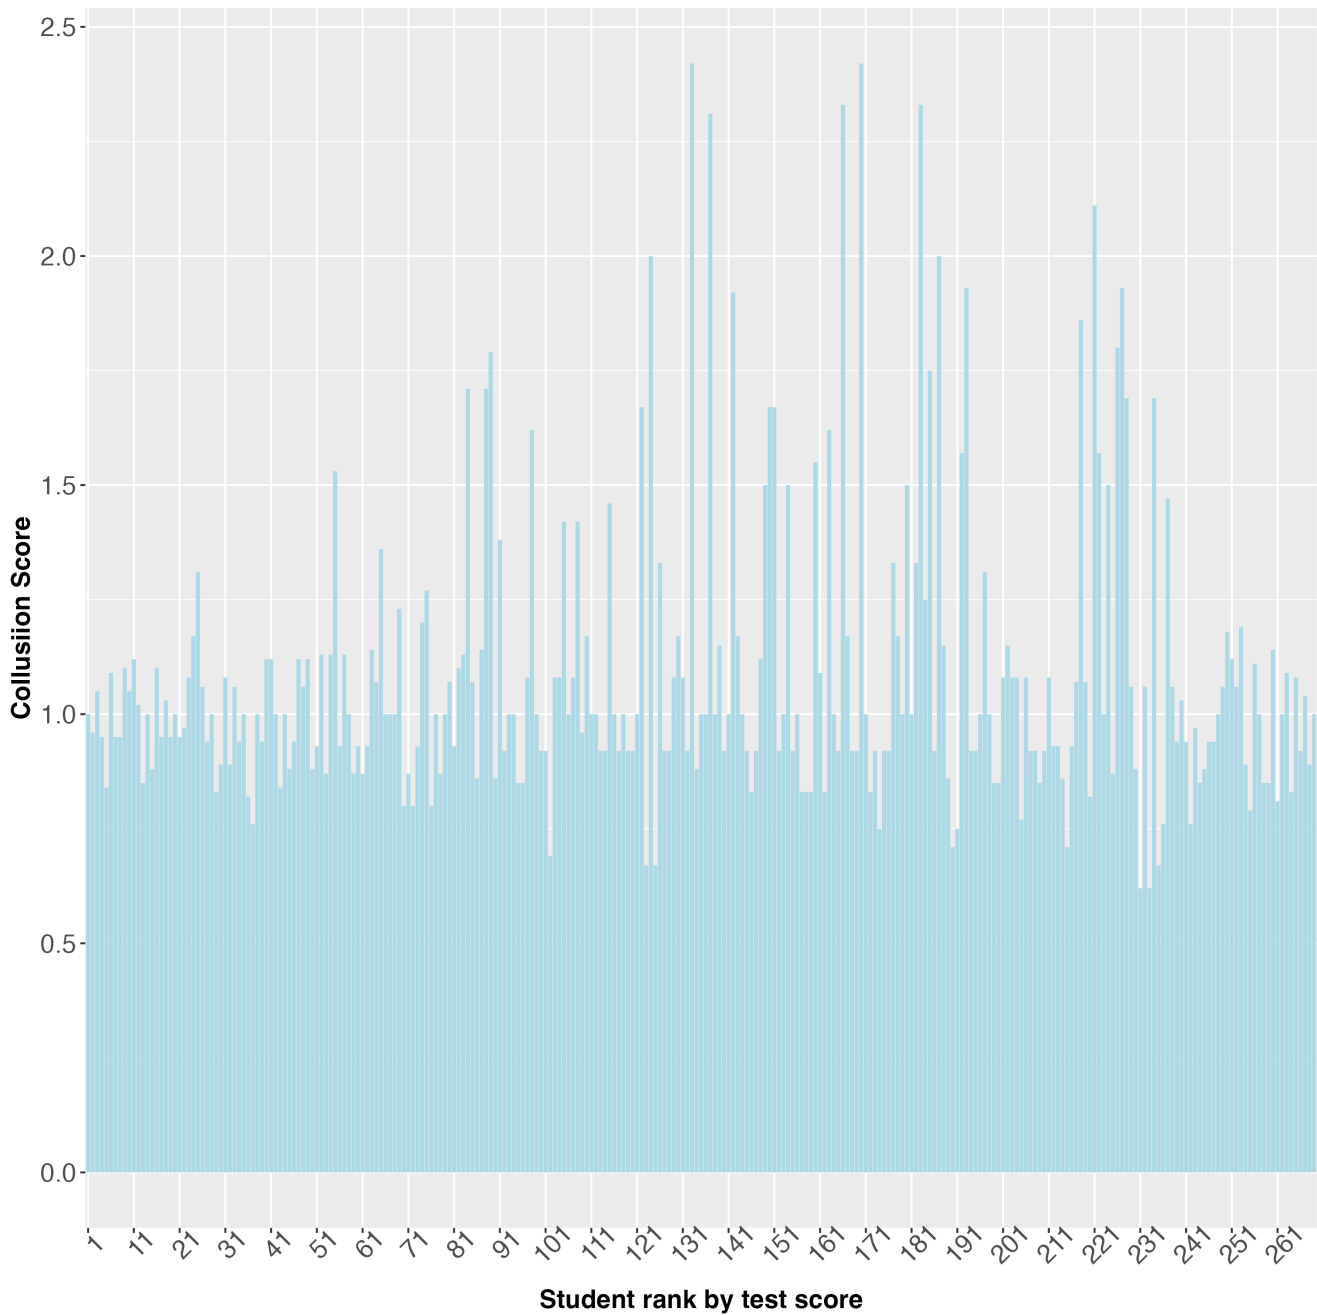

4. Histograms of Identity Scores (ISs) for one member of each Collusion Group

The Identity Score (IS) is the number of question scores that are identical between a pair of students. For each group, ISs are calculated between the group member with the highest CS and all other students who took the exam(s). Histograms of the frequency of ISs are shown below, one for each group. Pairs that include another member of the Collusion Group have higher ISs than pairs that include other students. As a result, pairs for which both members are part of the Collusion Group appear as outliers to the right of the main distribution.

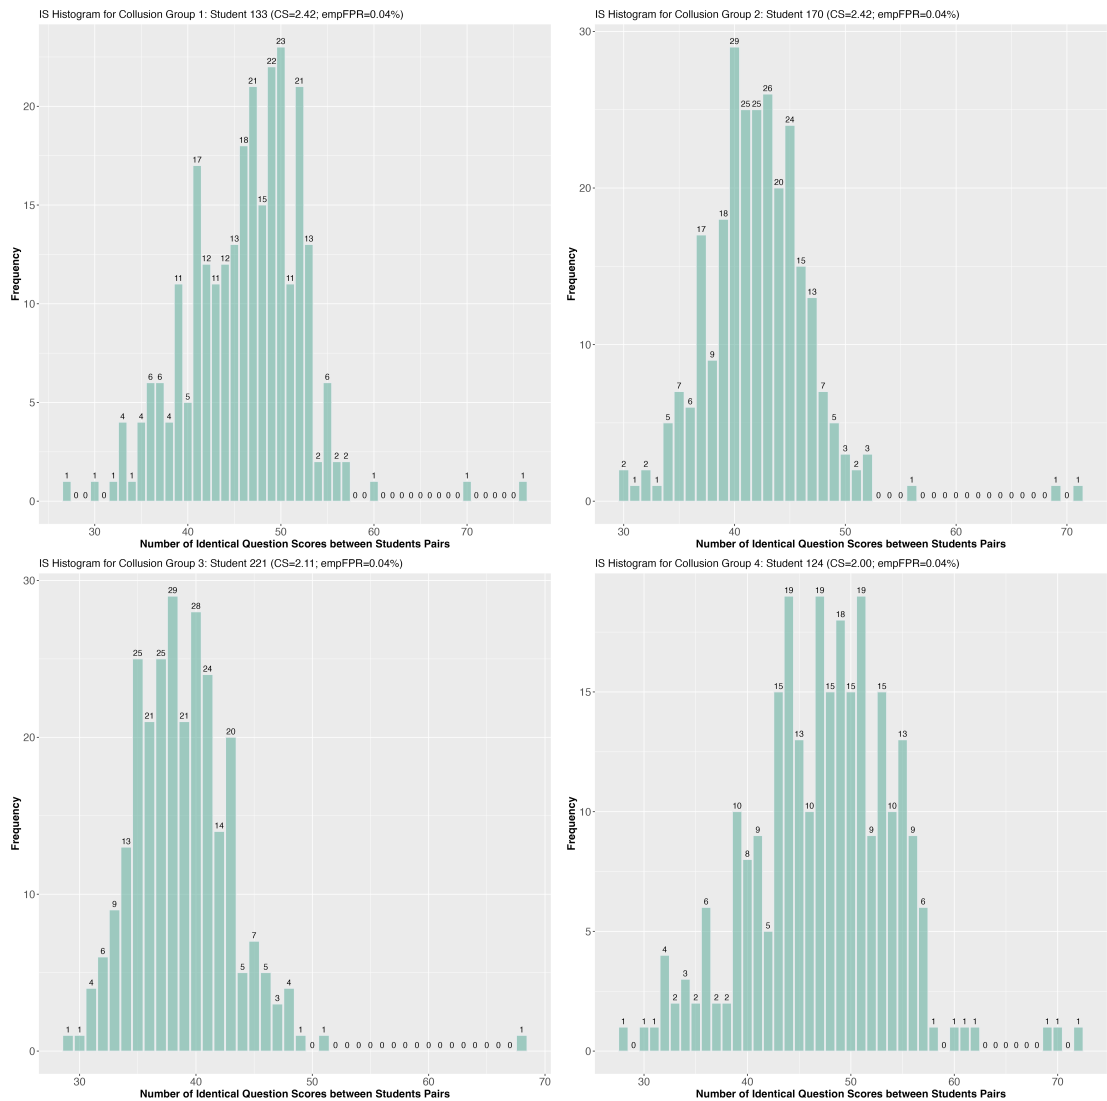



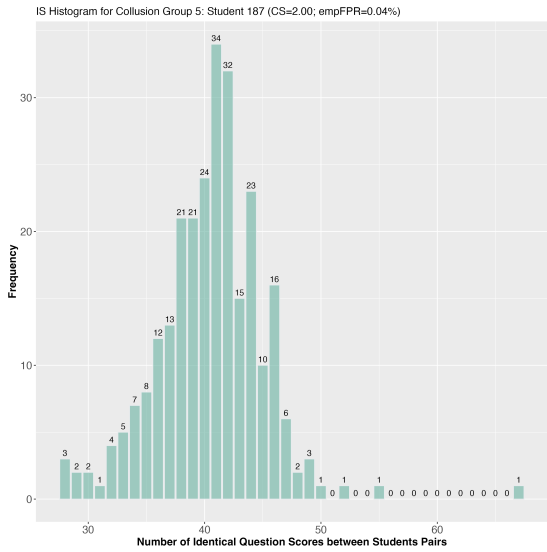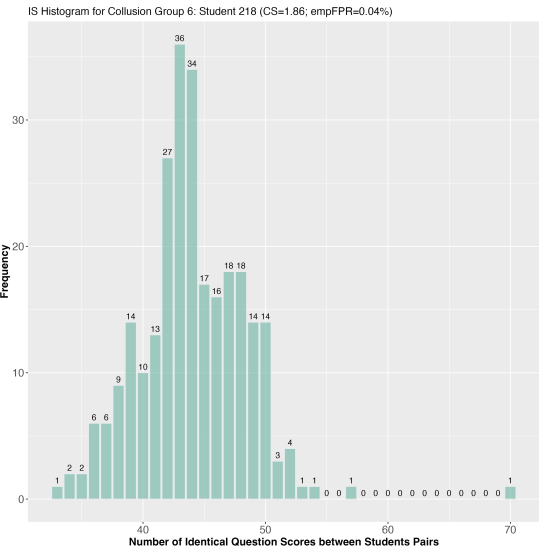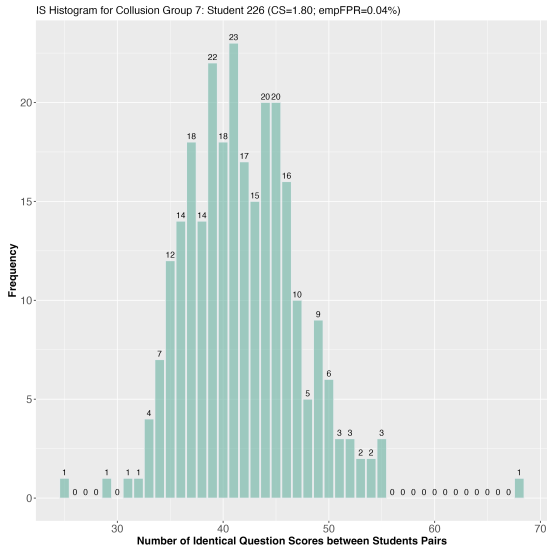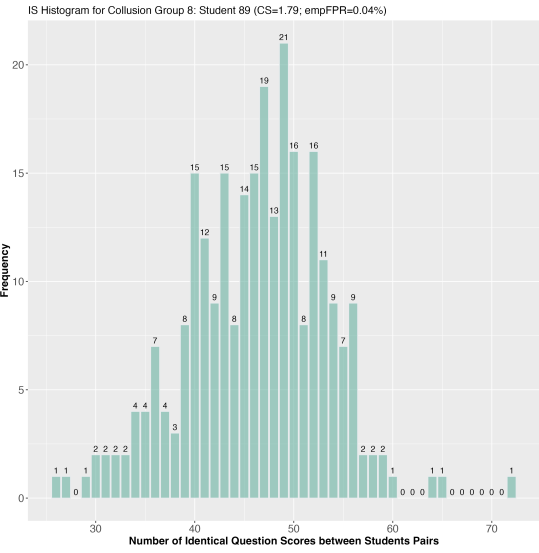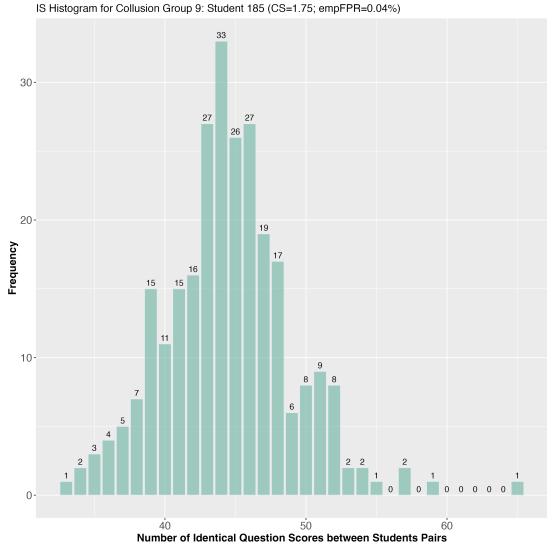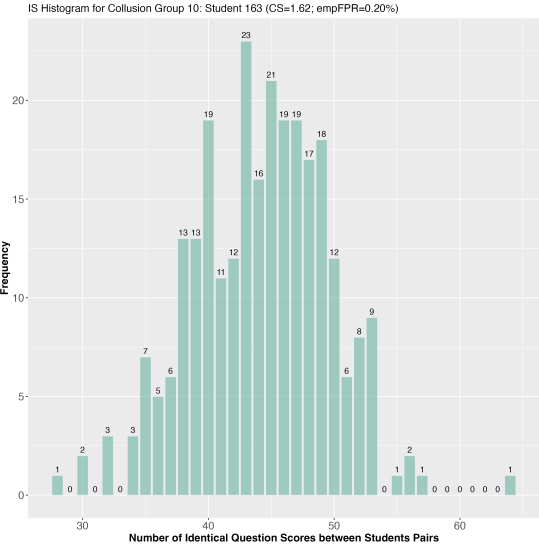

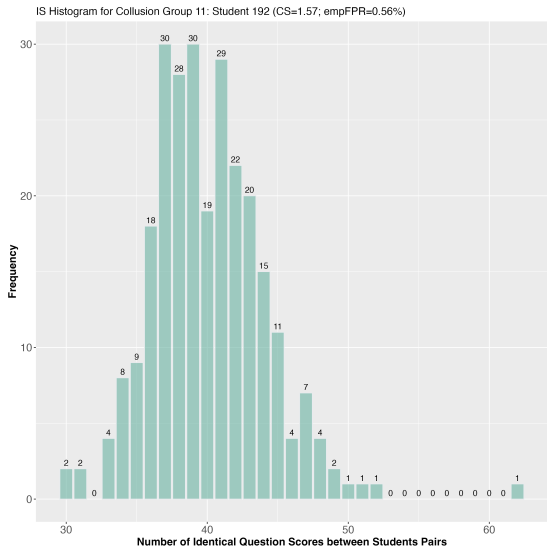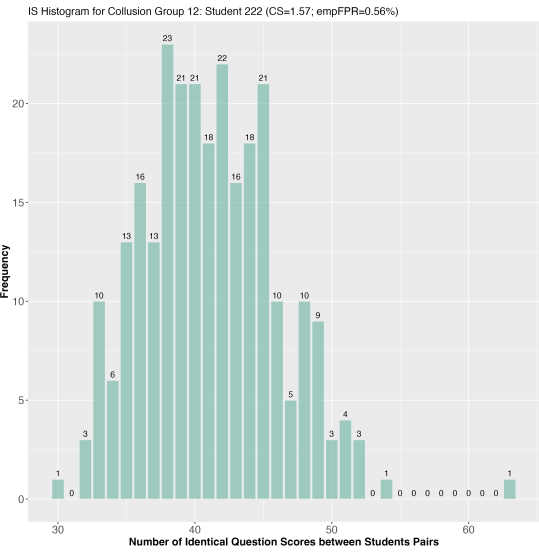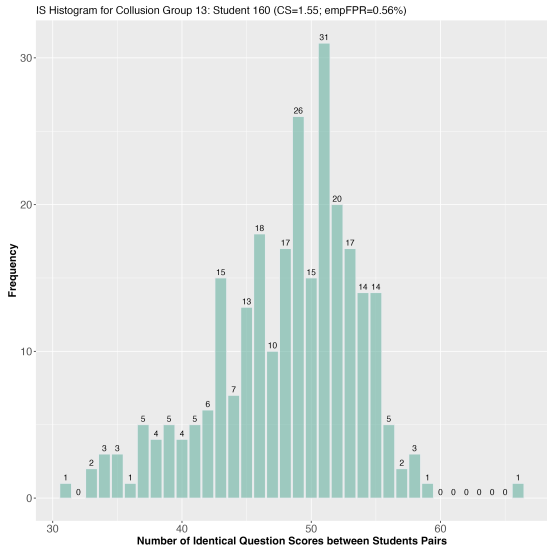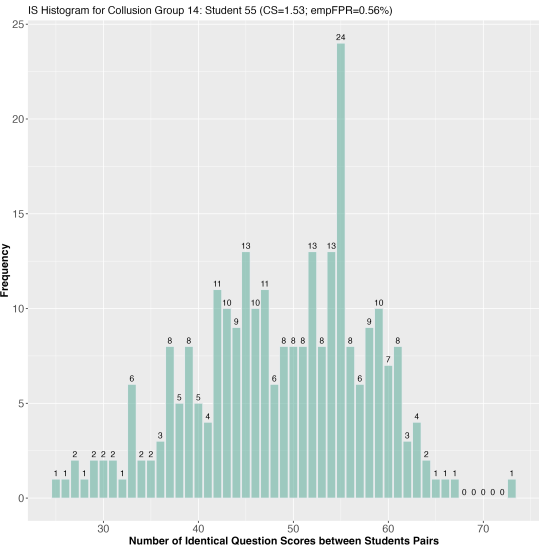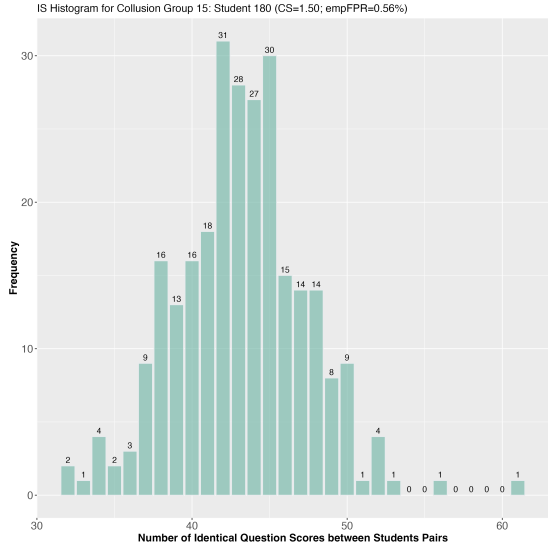

Supplement: Supplementary file 2 [file Q-SID Guide.pdf]
